# Supplementary material for: Multi-Dimensional Ability Diagnosis for Machine Learning Algorithms
Source: arXiv:2307.07134 source file (2023-07-14)
Supplement: Supplementary file 1 [file appendix.tex]

\section*{Appendix}

\begin{table*}[t]
    \scalebox{0.76}{
    \begin{tabular}{lccccc}
    \toprule
    \multirow{2}{*}{\textbf{Algorithm}} & \multirow{2}{*}{\textbf{Overall Accuracy}} & \multicolumn{4}{c}{\textbf{Top Skill}~(\emph{Ability Ranking})}  \\ 
    \cmidrule[0.5pt](r){3-6}
     &  & Top 1 & Top 2  & Top 3 & Top 4   \\
    \midrule
    Random Forest & 0.847 & Queenstown~(0.883) & Ticket Class 3rd~(0.726) & Ticket Class 1st~(0.705) & Southampton~(0.701) \\
    Decision Tree & 0.818  &  Ticket Class 1st~(0.895) & Southampton~(0.803) & Cherbourg~(0.713) &  Ticket Class 3rd~(0.678)         \\
    C-Support Vector Machine & 0.802  &  Ticket Class 3rd~(0.837) & Southampton~(0.790) & Queenstown~(0.774) &  Ticket Class 2nd~(0.725)   \\ \midrule
    Linear Support Vector Machine & 0.795  &  Queenstown~(0.824) & Ticket Class 3rd~(0.809) & Cherbourg~(0.768) &  Ticket Class 2nd~(0.754)     \\
    Gaussian Naive Bayes & 0.791  &  Ticket Class 2nd~(0.853) & Queenstown~(0.781) & Ticket Class 3rd~(0.760) &  Southampton~(0.758)   \\

    SGD Classifier  & 0.768 & Queenstown~(0.815) & Ticket Class 2nd~(0.796) & Ticket Class 1st~(0.738) & Southampton~(0.715)  \\

    K-Nearest Neighbors & 0.758  &  Ticket Class 2nd~(0.873) & Queenstown~(0.687) & Cherbourg~(0.675) &  Ticket Class 3rd~(0.621)    \\

    Perceptron & 0.732 & Southampto~(0.756) & Ticket Class 2nd~(0.728) & Queenstown~(0.694) & Ticket Class 3rd~(0.657) \\ \midrule
    
    Logistic Regression & 0.687  &  Cherbourg~(0.728) & Ticket Class 2nd~(0.692) & Queenstown~(0.680) &  Ticket Class 1st~(0.673)          \\
    \bottomrule
    \end{tabular}}
    
    \caption{Top-4 skills ranked by diagnostic metric \textit{Ability}  of 9 learners in Titanic. The table cells in the columns of \emph{Top Skill} denotes ``skill~(\emph{Ability})'', i.e., the skill and the corresponding \emph{Ability} performance.}
  
    \label{table: model_compare_titanic}
\end{table*}

\begin{table*}[t]
    \scalebox{0.855}{
    \begin{tabular}{lcccccc}
    \toprule
    \multirow{2}{*}{\textbf{Algorithm}} & \multirow{2}{*}{\textbf{Overall Accuracy}} & \multicolumn{5}{c}{\textbf{Top Skill}~(\emph{Ability Ranking})}  \\ 
    \cmidrule[0.5pt](r){3-7}
     &  & Top 1 & Top 2  & Top 3 & Top 4 & Top 5  \\
    \midrule
    
    ResNext50 & 0.563  &  palm tree~(0.870) & road~(0.852) & keyboard~(0.835) &  cup~(0.792)   &  pear~(0.790)              \\
    ResNext101 & 0.562  &  wardrobe~(0.963) & skyscraper~(0.881) & orchid~(0.880) &  chimpanzee~(0.797)   &  keyboard~(0.789)              \\
    % ResNet152 & 0.5386  &  orange~(0.836) & aquarium fish~(0.833) & wardrobe~(0.816) &  chair~(0.809)   &  bicycle~(0.803) \\
    DenseNet121 & 0.538  &  sunflower~(0.920) & orange~(0.884) & road~(0.876) &  chair~(0.858)   &  television~(0.819) \\
    ResNet18 & 0.532 &  sunflower~(0.904) & motorcycle~(0.856) & wardrobe~(0.853) &  tiger~(0.823)   &  butterfly~(0.755) \\
    WideResNet & 0.532  &  road~(0.948) & bicycle~(0.880) & mountain~(0.868) &  chair~(0.824)   &  bed~(0.804)              \\
    
    Xception & 0.530  &  apple~(0.941) & skunk~(0.861) & skyscraper~(0.842) &  chair~(0.827)   &  sunflower~(0.826)              \\

    ResNet101 & 0.529  &  poppy~(0.801) & road~(0.789) & apple~(0.786) &  rocket~(0.782)   &  keyboard~(0.779)              \\

     DenseNet161 & 0.528 & palm tree~(0.915) & keyboard~(0.869) & mountain~(0.840) & cockroach~(0.826) & skyscraper~(0.819) \\

     SeResNet34 & 0.516 & cockroach~(0.908) & bicycle~(0.872) & castle~(0.860) & whale~(0.824) & tiger~(0.818) \\

     ResNet152 & 0.516 & sunflower~(0.890) & raccoon~(0.856) & lion~(0.839) & plain~(0.809) & rose~(0.806) \\

    \bottomrule
    \end{tabular}}
    
    \caption{Top-5 skills ranked by diagnostic metric \textit{Ability}  of 10 learners in CIFAR-100. The table cells in the columns of \emph{Top Skill} denotes ``skill~(\emph{Ability})'', i.e., the skill and the corresponding \emph{Ability} performance.}

    \label{table: model_compare_cifar}
\end{table*}

In this section, we further report more detailed diagnostic interpretation results. 

\subsection*{Which skill is the learner good at?} 

% Due to the page limit, we compare two learner couples of CIFAR-100 and Titanic  in Figrue~\ref{Fig.compare_model} respectively. In this subsection, we further compare different learners of CIFAR-100 and Titanic respectively and their corresponding strength skills. For these two datasets, we obtain the overall \emph{Accuracy} score of each learner by evaluated it on the corresponding training set with 5-fold cross validation~\cite{browne2000cross}. Without loss of generality, we assess the \emph{Ability} of each learners for sample classes or features~(i.e. skills) by Eq.~(\ref{output}) and rank the strength skills of learners based on the \emph{Ability}.

In Figure~\ref{diagnose factor visualization}c~(in this paper), we demonstrate two learners, i.e., ResNet18 and DenseNet161 in CIFAR-100, Random Forest and K-Nearest Neighbors in Titanic, to show which skills they are good at in practice. In this subsection, we further conduct thorough analyses of learner \emph{Ability} performance. Specifically, we show more different categories of learners in both Titanic and CIFAR-100 respectively and their corresponding strength skills.

To set up this experiment, we first evaluate each learner in overall \emph{Accuracy} by 5-fold cross validation~\cite{browne2000cross} on the corresponding training set. Then we assess the \emph{Ability} of each learner for sample classes or features~(i.e. skills) by Eq.~(\ref{output}). Finally, we obtain the strength skills of learners based on the \emph{Ability}.

% Since massive traditional machine learning algorithms are applied to Titanic, we select 9 typical learners~(e.g. Random Forest, Decision Tree and C-Support Vector Machine) from whole 578 learners in Titanic and apprehend their performance difference. As shown in Table~\ref{table: model_compare_titanic}, we rank these learners based on their \emph{Accuracy} performance, and we investigate the strength skills of each learner ranked by \emph{Ability}. From Table~\ref{table: model_compare_titanic}, we have following finding. (1)~The learners based on tree structures~(i.e. Random Forest and Decision Tree) have the highest \emph{Accuracy} performance in Titanic. (2)~Each learner has different strengh skills. For example, though Random Forest have a best \emph{Accuracy} performance among these learners and have highest a \emph{Ability} value in samples of ``Queenstown'',  while Perceptron outperforms Random Forest in ``Southampto''. 

As for the learners, since massive traditional machine learning algorithms are applied to Titanic, we split the learners into groups according to overall \emph{Accuracy} performance for better interpretation. As shown in Table~\ref{table: model_compare_titanic}, we select 9 typical learners~(e.g. Random Forest, Decision Tree, and C-Support Vector Machine) from the whole 578 learners in Titanic and apprehend their \emph{Ability} performance difference. As for CIFAR-100, we compare strength skills of 10 learners with similar overall \emph{Accuracy} performance from 59 learners including many popular Convolution Neural Network~(e.g. ResNet and DenseNet) in Table~\ref{table: model_compare_cifar}. 

We have the following findings from Table~\ref{table: model_compare_titanic} and Table~\ref{table: model_compare_cifar}. (1) Each learner has different strengh skills. For instance, in Table~\ref{table: model_compare_titanic}, though Random Forest have a best \emph{Accuracy} performance among these learners and have highest a \emph{Ability} value in samples of ``Queenstown'',  while Perceptron outperforms Random Forest in ``Southampto''.  (2) Though learners may have similar overall \emph{Accuracy} performance, the strength skills of different learners vary greatly. For example, as shown in Table~\ref{table: model_compare_cifar}, even if ResNet18 and WideResNet have a same overall \emph{Accuracy}  score, ResNet is adept at the ``sunflower'' class while WiderResNet specializes in the ``road'' class.

\subsection*{Which learners have the highest \emph{Ability} in specific skills?}
In the areas of algorithm combinations~\cite{duh2011generalized}, researchers may pay more attention to the question: when given a specific skill~(e.g. sample category features or sample class labels), which learners have the highest performance on it? To answer this question,  in Table~\ref{table: skill_compare_cifar}, we randomly select 10 skills and corresponding learners with highest \emph{Ability}. We acquire the learners' \emph{Ability} values on the specific skills via Eq.~(\ref{output}). We can see that as for each skill, the learners with the highest \emph{Ability} are very different. For example, Inceptionv4 has the highest \emph{Ability} performance in the ``Cloud'' skill according to \emph{Ability}, while WiderResNet is the best in predict the ``Bicycle'' skill. Such diagnostic results for each skill and corresponding learners with highest \emph{Ability} performance can provide detailed information for algorithm analysis and algorithm combinations.

\begin{table*}[t]
    \scalebox{0.74}{
    \begin{tabular}{lcccccc}
    \toprule
    \multirow{2}{*}{\textbf{Skill}} & \multirow{2}{*}{\textbf{Overall Accuracy}} & \multicolumn{5}{c}{\textbf{Top Learner}~(\emph{Ability Ranking})}  \\ 
    \cmidrule[0.5pt](r){3-7} 
    & & Top 1 & Top 2  & Top 3 & Top 4 & Top 5 \\
    \midrule
    Cloud & 0.630  &  Inceptionv4~(0.800) & PreActResNet~(0.761) & ShuffleNet~(0.760) &  SqueezeNet~(0.754)   &  ResNext101~(0.740)              \\
    Bicycle & 0.726  &  WiderResNet~(0.820) & SeResNet~(0.805) & ResNet152~(0.802) &  DenseNet161~(0.780)   &  ResNext101~(0.748)              \\
    
    Tank & 0.562  &  ResNext101~(0.779) & ResNet152~(0.744) & WiderResNet~(0.715) &  ResNet18~(0.698)   &  DenseNet161~(0.693) \\
    Palm tree & 0.718  &  DenseNet161~(0.878) & ResNext50~(0.870) & StochasticDepth101~(0.853) &  SeResNet18~(0.840)   &  SeResNet50~(0.794) \\
    Wolf & 0.442  &  ResNet152~(0.685) & ResNet101~(0.677) & NasNet~(0.669) &  DenseNet201~(0.660)   &  DenseNet121~(0.652)              \\
    
    Fox & 0.326  &  DenseNet161~(0.726) & ResNet101~(0.674) & DenseNet121~(0.669) &  SeResNet18~(0.666)   &  Xception~(0.651)              \\

    Can & 0.522  &  DenseNet161~(0.843) & WiderResNet~(0.678) & ResNext50~(0.677) &  ResNext101~(0.658)   &  SeResNet18~(0.657)              \\

     Rose & 0.634 & ResNext152~(0.740) & WiderResNet~(0.739) & DenseNet161~(0.727) & ResNext50~(0.725) & StochasticDepth101~(0.715) \\

     Rabbit & 0.470 & ResNext101~(0.720) & DenseNet161~(0.658) & ResNet18~(0.626) & NasNet~(0.608) & ResNet101~(0.604) \\

     Leopard & 0.562 & ResNext152~(0.740) & ResNext50~(0.689) & ResNet101~(0.689) & Xception~(0.686) & DenseNet201~(0.675) \\
    
    % WideResNet & 0.5317 & road~(0.948/0.894) & bicycle~(0.880/0.800) & bear~(0.362/0.198) &  seal~(0.253/0.128)  \\
    % Xception & 0.5296 & apple~(0.941/0.854) & skunk~(0.861/0.792)  & tank~(0.383/0.418) &  man~(0.344/0.200)  \\
    % DenseNet121 & 0.5282 & palm tree~(0.915/0.836) & keyboard~(0.869/0.786) & otter~(0.302/0.122) &  girl~(0.299/0.166)  \\
    % SeResNet34 & 0.5160 & cockroach~(0.908/0.840) & bicycle~(0.872/0.782) & chimpanzee~(0.363/0.390) &  lizard~(0.289/0.184)  \\
    \bottomrule
    \end{tabular}}
    \caption{Top-5 learners ranked by diagnostic metric \textit{Ability}  of 10 skills in CIFAR-100. The table cells in the columns of \emph{Top Learner} denotes ``learner~(\emph{Ability})'', i.e., the learner and the corresponding \emph{Ability} performance on the skill~(first column).}
    \label{table: skill_compare_cifar}
\end{table*}

\begin{figure}[t]
    \centering %图片居中
    \includegraphics[width=0.4\textwidth]{Figures/visualize_q.pdf}
    \caption{t-SNE visualization of sample skill mask factor and corresponding skill annotations in CIFAR-100.}
    \label{Fig.visualize_q}
\end{figure}

\subsection*{What is the relation between latent sample skill mask factors and explicit skills?} 

% To handle the machine learning tasks without explicit sample-skill matrix, our proposed diagnostic framework \emph{Camilla} can utilize sample skill mask factors~(Eq.~(5)) to  models the association of samples and skills implicitly. In this subsection, we empirically show that the latent sample skill mask factor can cluster the samples with similar features like explicit class labels, and have other merit which explicit skills do not have.

In our proposed diagnostic framework \emph{Camilla}, one of the most important merits is that we do not need an explicit sample-skill matrix as input. Please revisit Figure~\ref{Fig.model} and Section 4 for more intuitive and detailed descriptions of the sample-skill matrix. \emph{Camilla} can learn the implicit relation between samples and skills automatically through Eq.~(5), hence \emph{Camilla} has more flexible and extensive applicability in various machine learning tasks. In this subsection, we conduct a detailed analysis to prove the correlation between implicit sample-skill relationship learned by our \emph{Camilla} and explicit skill annotations of samples. Specifically, we carry out experiments on CIFAR-100, since this dataset has clear skill annotations. 

% As shown in Figure~\ref{Fig.visualize_q}, we visualize the sample skill mask factors of \emph{Camilla-PM} in ``Elephant'', ``Lion'' and ``Tiger'' classes of CIFAR-100. In Figure~\ref{Fig.visualize_q}, the sample skill mask factors of each class are relatively and centrally distributed. It illustrates that through the response logs from learners to samples and pre-trained representations of samples, the skill mask factors of our diagnoser \emph{Camilla-PM} can represent the explicit skill~(e.g. classes) of samples approximately.

We randomly select 3 image classes~(e.g. ``Elephant'', ``Lion'' and ``Tiger''), which we view as explicit skills, and 500 samples for each in CIFAR-100. Then we project their sample \emph{skill mask} factors~(Eq.~(5)) of \emph{Camilla-PM} into 2D space by t-SNE for visualization in Figure~\ref{Fig.visualize_q}. We mark the samples with their class labels using different colors. As shown in Figure~\ref{Fig.visualize_q}, the sample \emph{skill mask} factors of each class are relatively and centrally distributed. It illustrates that through the response logs from learners to samples and pre-trained representations of samples, the \emph{skill mask} factors of our diagnoser \emph{Camilla-PM} can represent the explicit skill~(e.g. classes) of samples approximately.

Furthermore, we select 6 samples from the center of the \emph{skill mask} factors in the three image classes~(i.e. ``Elephant'', ``Lion'' and ``Tiger''). We can see that the images whose \emph{skill mask} factors are located in the center of several image classes have a high \emph{difficulty} factor, and their inherent features are ambiguous. For example, in Figure~\ref{Fig.appendix_case}, the ``Tiger'' sample has a highest \emph{difficulty} value and it contains a complex scenario~(i.e. many gray trees) and a fuzzy outline of ``tiger". And the ``Lion'' sample with 0.90 \emph{difficulty} value is easy to be identified wrongly as ``Tiger''. Compared to the explicit skill~(e.g. classes), latent \emph{skill mask} factors not only aggregate the samples which have similar inherent features, but also reflect the  ambiguous features of samples.

\begin{figure}[]
    \centering %图片居中
    \includegraphics[width=0.47\textwidth]{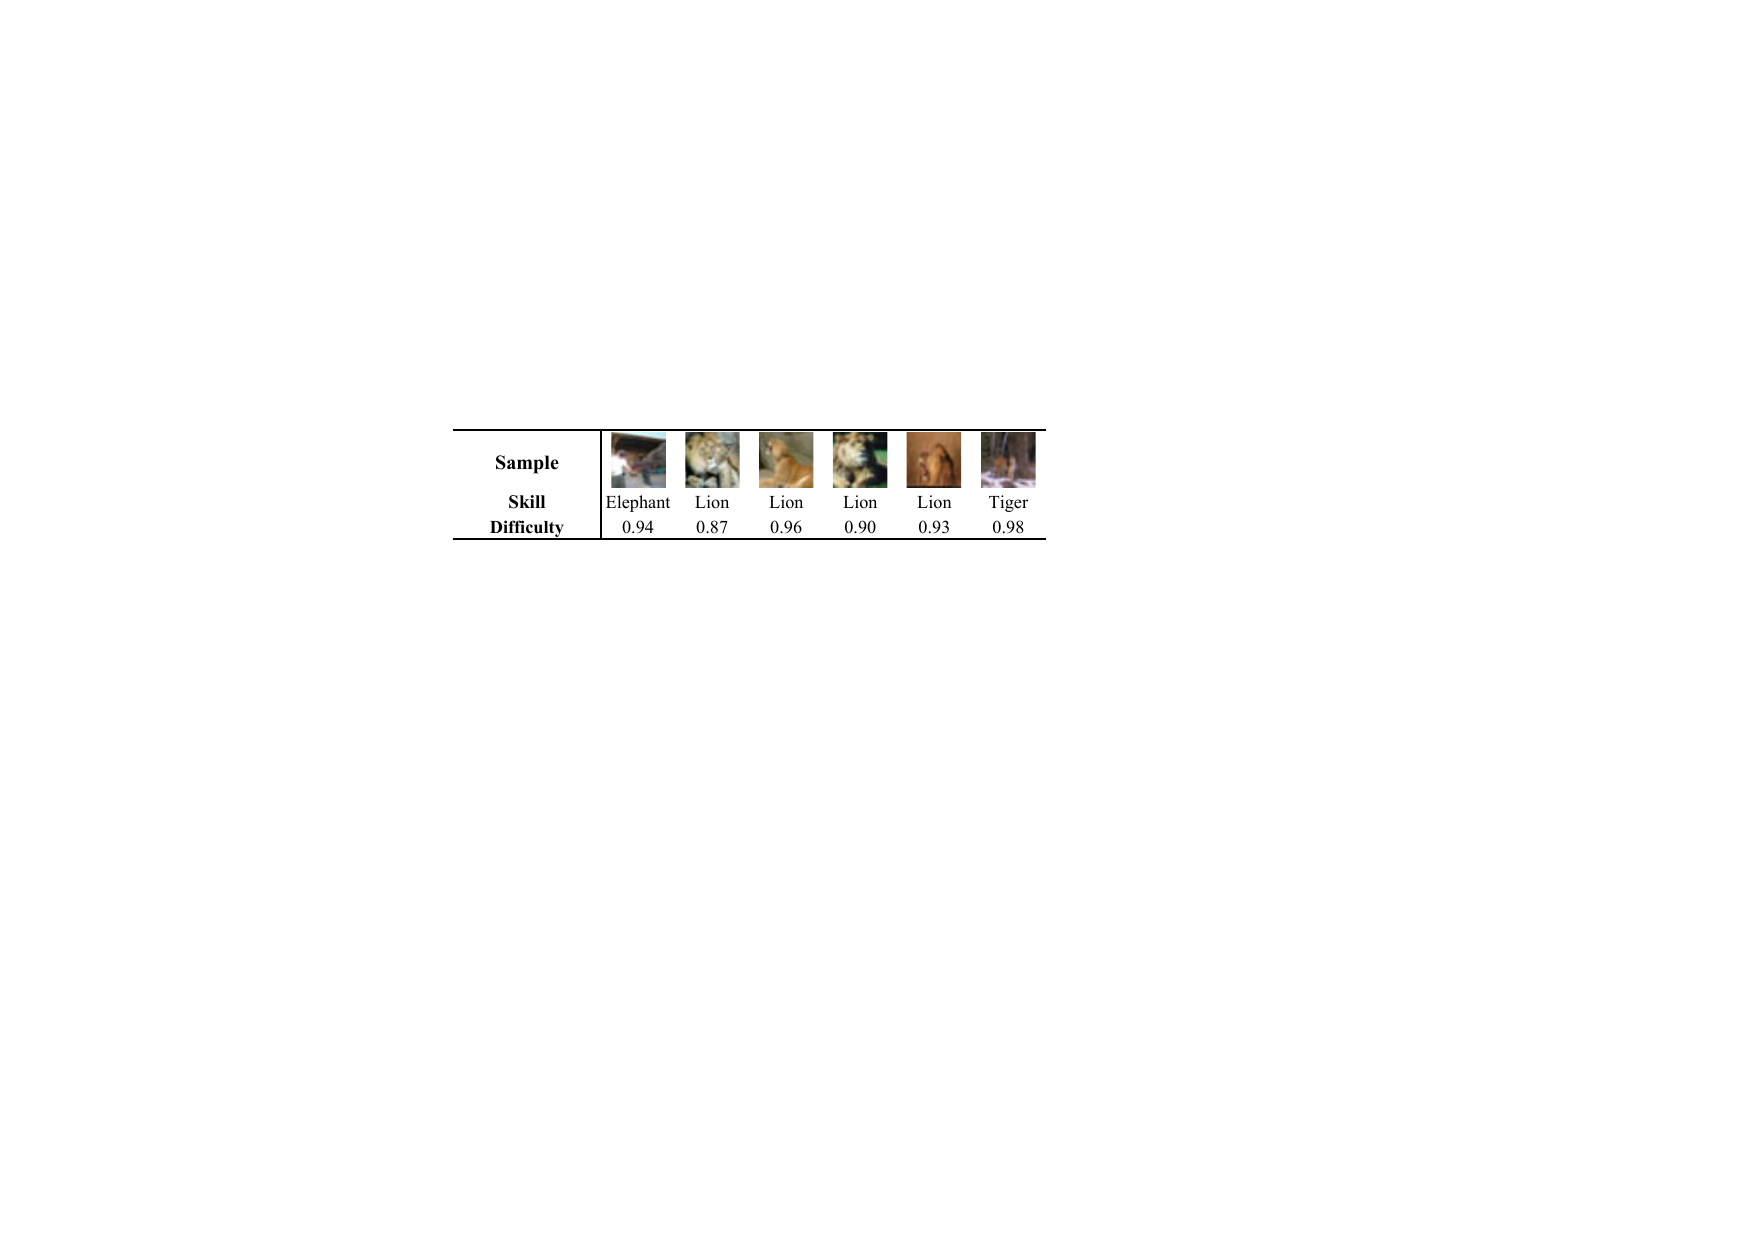}
    \caption{The samples whose \emph{skill mask} factors are located in the center of the three classes and the corresponding skills and difficulty factors.
    }
    \label{Fig.appendix_case}
\end{figure}

% \begin{figure}[ht]
%     \centering
%     \subfigure[]{
%     \begin{minipage}{1\linewidth}
%     \centering
%     \includegraphics[width=3in]{Figures/visualize_q.pdf}
%     \end{minipage}%
%     }%

%     \subfigure[]{
%     \begin{minipage}{1\linewidth}
%     \centering
%     \includegraphics[width=3in]{Figures/appendix_case.pdf}
%     \end{minipage}%
%     }%
%     \centering
%     \caption{Individual learner performance on different classes of CIFAR100~(Left Figure). \emph{Jaccard} similarity of two learners' responses in CIFAR-100~(Right Figure).}
%     \label{Fig.last_case}
% \end{figure}
